# Supplementary material for: Signature of pressure-induced topological phase transition in ZrTe$_5$
Source: arXiv:2312.10223 ancillary file (2024-10-28)
Supplement: Supplementary file 1 [file suppinfo_Signature-Pressure-ZrTe5_KovacsKrausz_et_al.pdf]

# Supporting Information: Signature of pressure-induced topological phase transition in $\text{ZrTe}_5$

Zoltán Kovács-Krausz,<sup>1,2</sup> Dániel Nagy,<sup>3</sup> Albin Márfy,<sup>1,2</sup> Bogdan Karpiak,<sup>4</sup>  
Zoltán Tajkov,<sup>5,6</sup> László Oroszlány,<sup>3,7</sup> János Koltai,<sup>8</sup> Péter Nemes-Incze,<sup>5</sup>  
Saroj P. Dash,<sup>4</sup> Péter Makk,<sup>1,9,\*</sup> Szabolcs Csonka,<sup>1,2</sup> and Endre Tóvári<sup>1,9</sup>

<sup>1</sup>*Department of Physics, Institute of Physics,  
Budapest University of Technology and Economics, H-1111 Budapest, Hungary*

<sup>2</sup>*MTA-BME Superconducting Nanoelectronics  
Momentum Research Group, H-1111 Budapest, Hungary*

<sup>3</sup>*Department of Physics of Complex Systems,  
ELTE Eötvös Loránd University, 1117 Budapest, Hungary*

<sup>4</sup>*Department of Microtechnology and Nanoscience,  
Chalmers University of Technology, SE-41296, Göteborg, Sweden*

<sup>5</sup>*Hungarian Research Network, Centre for Energy Research,  
Institute of Technical Physics and Materials Science, 1121 Budapest, Hungary*

<sup>6</sup>*Centre of Low Temperature Physics, Institute of Experimental Physics,  
Slovak Academy of Sciences, Košice SK-04001, Slovakia*

<sup>7</sup>*MTA-BME Lendület Topology and Correlation Research Group,  
Budapest University of Technology and Economics, 1521 Budapest, Hungary*

<sup>8</sup>*Department of Biological Physics, ELTE Eötvös  
Loránd University, 1117 Budapest, Hungary*

<sup>9</sup>*MTA-BME Correlated van der Waals Structures  
Momentum Research Group, H-1111 Budapest, Hungary*

## I. MAGNETOTRANSPORT IN ADDITIONAL DEVICES

We present additional magnetotransport measurement sets in the full temperature range for additional devices in the 50 – 150 nm thickness range in Fig. S1 at pressures of 0 and 2 GPa. Each column is a different device. Overall, the individual measurements on each device are consistent with the pressure dependence behavior of device S2, presented in the main text. The  $R_{xx}$  traces are clearly flattened under pressure, while for the  $R_{xy}$  curves the sharp change in slope around a field value of 1 T vanishes. The latter is most visible at the lowest temperatures (blue curves). In addition, the Shubnikov-de Haas oscillations appear to be suppressed with pressure.

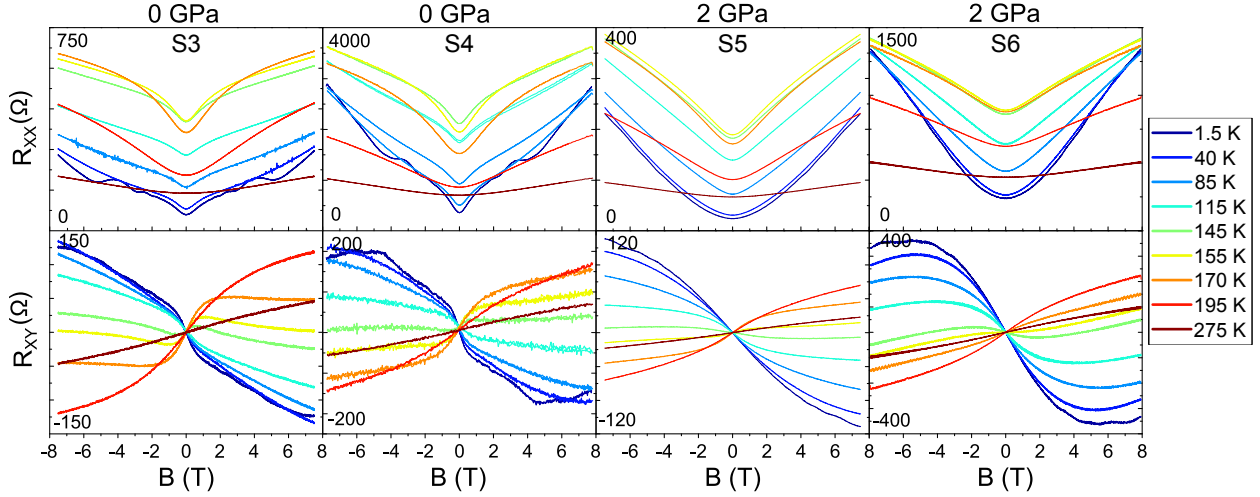

Figure S1. Additional magnetotransport measurements on  $\text{ZrTe}_5$  devices in the 50 – 150 nm thickness range, with two measurement sets without applied pressure and two sets at 2 GPa pressure. Each set is from a different device.

## II. PRESSURE DEPENDENT MULTICARRIER DETAILS

In Fig. S2 we demonstrate the pressure evolution of the MCT fitting results on sample S2 in detail at two representative temperatures. The top row (Fig. S2 (a)-(e)) shows the contribution of carriers at  $T = 40$  K, a temperature where the significant carrier contributions are from the conduction bands, but still high enough to avoid effects of Shubnikov-de Haas

\* makk.peter@ttk.bme.hu

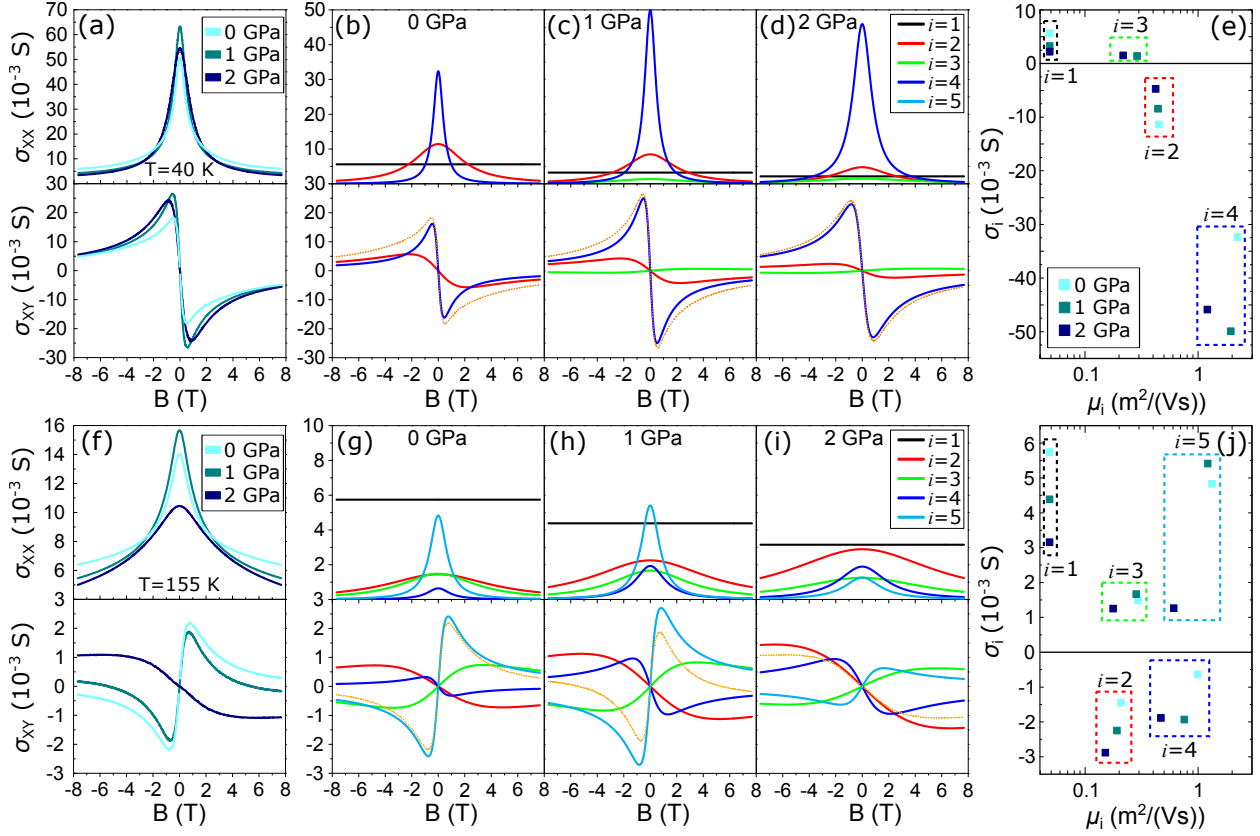

Figure S2. (a)  $\sigma_{xx}$  and  $\sigma_{xy}$  of sample S2 at  $T = 40$  K for three studied pressures. (b)-(d) Individual carrier contributions to  $\sigma_{xx}$  and  $\sigma_{xy}$  at 0, 1 and 2 GPa, respectively, obtained from MCT fitting. For the  $\sigma_{xy}$  their sum is also plotted (orange dotted line), identical to the curves in (a). (e) The change of the  $\sigma_i$  (signed: positive for holes and  $\sigma_1$ , negative for electrons) and  $\mu_i$  parameters of each carrier as a function of pressure. Each carrier is grouped into a color-coded box. (f)-(j) The same respective plots at  $T = 155$  K. Note that, in panels (e), (j), the mobility scale is logarithmic, but  $\mu_1 = 0$  is plotted at the minimum of the scale for the sake of representing  $\sigma_1$  on the plot.

oscillations. Panels (b)-(d) show the decomposition of conductivity into the various carrier contributions obtained from the fitting process. The horizontal black line in the  $\sigma_{xx}$  panels is the edge carrier ( $i = 1$ ), the contribution of which can be seen to decrease with pressure. The predominant  $\sigma$  contributions are from the electron bands ( $i = 2, 4$ ). Their significantly different mobilities explain the sharp change in slope of  $R_{xy}$  around  $B = \pm 1$  T. At higher pressures the hole type carrier ( $i = 3$ ) appears, but its contribution remains small. The previously seen simplification (in the main text and in Fig. S1) of  $R_{xx}$  and  $R_{xy}$  curves at 2

GPa is to be expected as the transport becomes more dominated by one particular carrier ( $i = 4$ ).

The bottom row (Fig. S2 (f)-(j)) shows the results of the same procedure at a temperature of  $T = 155$  K, close to the  $T_p = 152$  K value of sample S2. While  $T_p$  itself is somewhat pressure-dependent as seen in the main text, the observed changes in carrier contributions cannot be explained by it. We see that the contribution of the  $i = 2$  carrier increases monotonically while that of the  $i = 3$  carrier, of comparable mobility, remains largely unchanged. The change in  $\sigma_i$  of the Dirac-like carriers are both non-monotonic; interestingly, from 0 to 1 GPa the electron-type  $|\sigma_4|$  increases more significantly compared to the hole-type  $\sigma_5$ , while from 1 to 2 GPa the opposite happens, with  $\sigma_5$  decreasing significantly while  $|\sigma_4|$  barely changes. Notably, the predominant carrier type changes from holes to electrons as the pressure is increased to 2 GPa. This can best be seen in the  $\sigma_{xy}$  dependence which clearly changes sign. As in the 40 K case, and in most of the temperature range, the edge carrier contribution gradually reduces with pressure.

### III. THICKNESS DEPENDENCE OF MAGNETOTRANSPORT

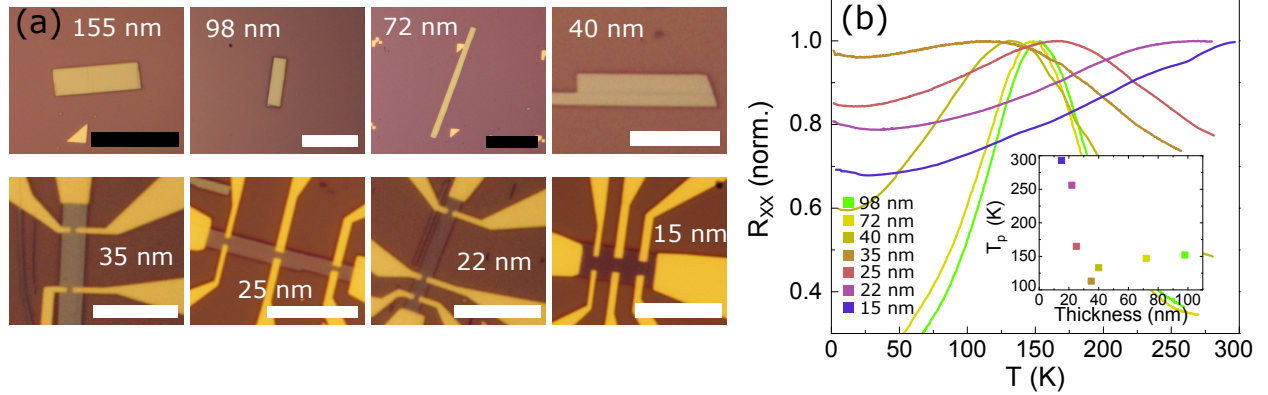

Figure S3. (a) Optical images of experimental ZrTe<sub>5</sub> devices on SiO<sub>2</sub>, with decreasing thickness inscribed in each image. Black (white) scale bars for reference are 25 (10)  $\mu$ m. (b) Anomalous resistivity peak and overall  $R_{xx}(T)$  dependence (normalized to maximum value) for different thicknesses. The inset is the extracted position of  $T_p$  with thickness from the main panel.

The signature of the phase transition was studied in detail on device S2 (98 nm thick)

in the main text. In the 50 – 150 nm range the studied devices show similar transport with temperature. Thickness-dependent effects start being relevant below 50 nm. We have studied a number of devices in this range as well. Fig. S3 (a) shows optical microscopy images of some of the devices, where a change in color with thickness can be observed. The characteristic  $R_{xx}(T)$  curves change significantly with decreasing thickness, as can be seen in Fig. S3 (b), similar to previous studies [1–3]. We can observe a nonmonotonic shift, with the peak position initially decreasing, after which the curve becomes flatter and the peak starts rapidly shifting upwards toward 300 K. The reversal of the trend in  $T_p$  takes place somewhere between 35 and 40 nm. This process can be better seen in the inset of panel (b), where the  $T_p$  values are extracted as discrete datapoints. This thickness dependence is remarkably consistent with that of Ref. [3], but at the same time contradictory with that seen in Ref. [2], which shows a monotonic thickness dependence for  $T_p$ .

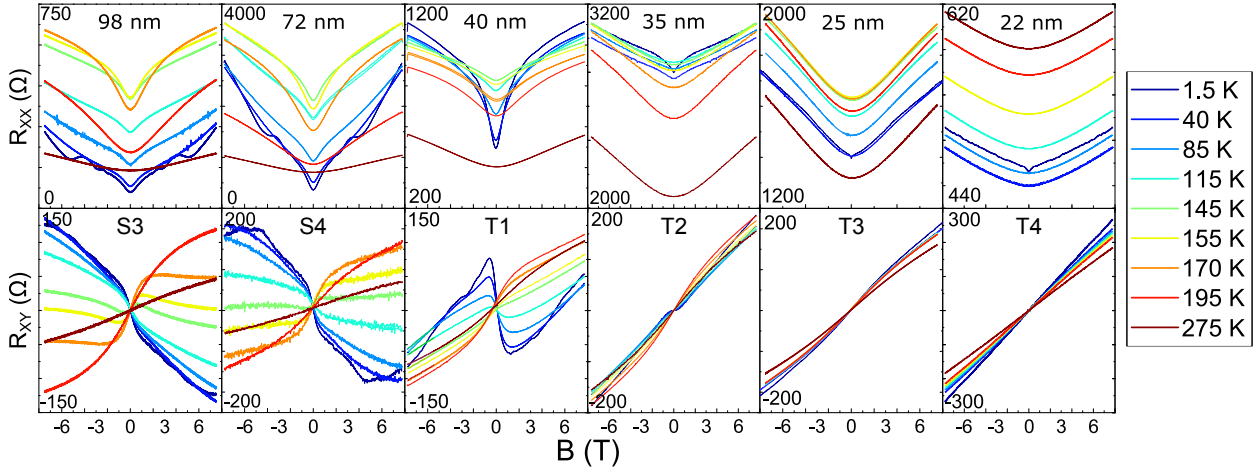

Figure S4. Thickness dependence of magnetotransport features, with decreasing thickness from left to right. As the thickness is reduced, the conduction band contributions at lower temperatures gradually disappear, with thinner devices having hole-dominant transport at all temperatures.

An extract of magnetotransport measurements on the thinner samples (T1-T4) are shown in Fig. S4. Only a few selected temperatures are displayed; many more temperatures were actually measured. The y-axis has been independently scaled for each panel to fit the data (note the y-axis limits written in the corners), so that the features of the curves at different thicknesses can be visually compared. The  $R_{xx}$  curves simplify as the thickness decreases, and start approaching parabolic-looking shapes. Below 40 nm thickness, the  $R_{xx}(B)$  traces

close to  $T_p$  no longer feature an increase in slope at low field values. In addition, with decreasing thickness, the signs of Shubnikov-de Haas oscillation exhibited at low temperature vanish. More importantly, in the  $R_{xy}$  traces the negative slope sections (suggesting electron-like transport from the regular Hall effect) are reduced in thinner devices, and are essentially absent in devices T3 and T4. Despite this, the curves remain nonlinear, even in case of device T4, suggesting continued multicarrier transport.

#### IV. THICKNESS DEPENDENCE OF BAND FITTING

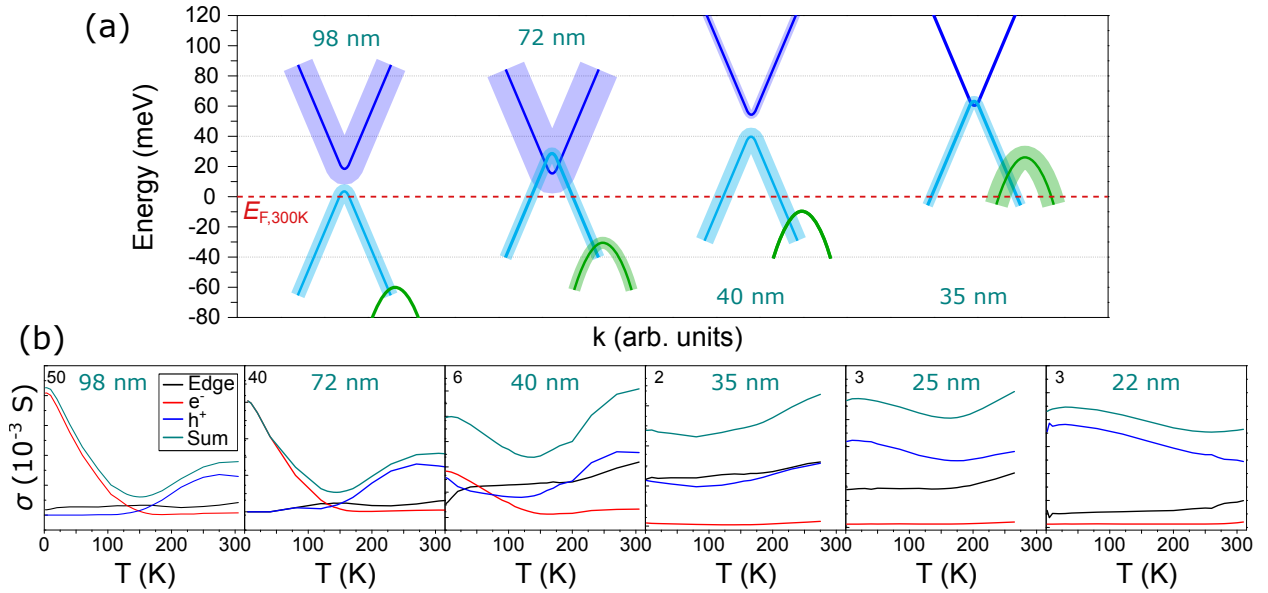

Figure S5. (a) Representation of the obtained band model from the MCT results, as a function of thickness. The error is represented by the thickness of the lines. There is an overall upward shift of all the band edge energies. The reference energy ( $E_{F,300K} = 0$  meV) is the chemical potential at 300 K. (b) Absolute conductivity contributions of the edge carrier (black), all electron carriers (red), all hole carriers (blue) and their sum (teal), as a function of temperature. The y-axes are scaled in each panel to fit the plots. The numbers in upper left of each panel are the top of the scale in  $10^{-3}$  S. The position of the minimum in the teal curve corresponds to the measured  $R(T)$  peak.

By fitting the  $n_{3D,i}(T)$  results from the MCT model, as in the main text, we can obtain the position of the band edges of the thinner samples as well. We notice a shift of the

chemical potential deeper into the valence band, as shown in Fig. S5 (a). This can be used to explain the initial downward shift of  $T_p$  from Fig. S3 (b), down to a thickness of around 40 nm (sample T1). The band edges being situated at higher energies means that the shifting chemical potential with temperature passes the gap in the Dirac-like bands at a lower temperature. This can also be discerned in Fig. S5 (b), showing the total conductivity compared to the electron and hole conductivity contributions respectively. Down to 40 nm, the minimum of conductivity in the teal curve (corresponding to the resistivity peak) moves downward in temperature along with the crossing point between electron and hole contributions (red and blue curves). For thinner devices (right side of Fig. S5 (b)), the chemical potential never crosses the gap. The conductivity minimum is instead given by the hole contribution, itself being a sum of the two different hole-type carriers.

## V. PRESSURE EFFECT ON THIN DEVICE

Here we present the magnetotransport and MCT modeling results, at 0 GPa and 2 GPa, for device T4 which is 22 nm thick. The thin devices feature a room-temperature pressure dependence of  $R_{xx}$  which is similar to thicker samples, as shown in Fig. S6 (a). In device T4 the minimum in  $R_{xx}$  is at a slightly increased pressure of around 1 GPa. As already seen in Fig. S4, 0 GPa measurements in this device show close to linear  $R_{xy}(B)$  traces at all temperatures. In comparison, the magnetotransport at 2 GPa shows more noticeable nonlinearity, as shown in Fig. S6 (b), for a few select temperatures. The MCT fitting results presented in Fig. S6 (c) and (d), show only small changes in the carrier properties with pressure. The edge carrier contribution ( $i = 1$ ) is slightly increased. As expected, the results show hole-dominated transport throughout the temperature range. At pressure, the dominant ( $i = 3$ ) carrier contribution slightly reduces and the minority ( $i = 5$ ) hole contribution increases. Because the latter consists of higher mobility carriers, this explains the increased nonlinearity of the low-temperature 2 GPa curves from Fig. S6 (b). Finally, the electron contribution is still present and features the highest mobility of all carriers. The magnitude of the conductivity contribution  $\sigma_4$  (in the inset of Fig. S6 (c)) is nonzero at all temperatures, but it is approximately an order of magnitude smaller than the  $\sigma_1$  and  $\sigma_5$  contributions, and there is no notable change with pressure. Unfortunately, the band fitting procedure on the MCT results for device T4 is not feasible. The  $n_{3D,i}(T)$  dependences are too

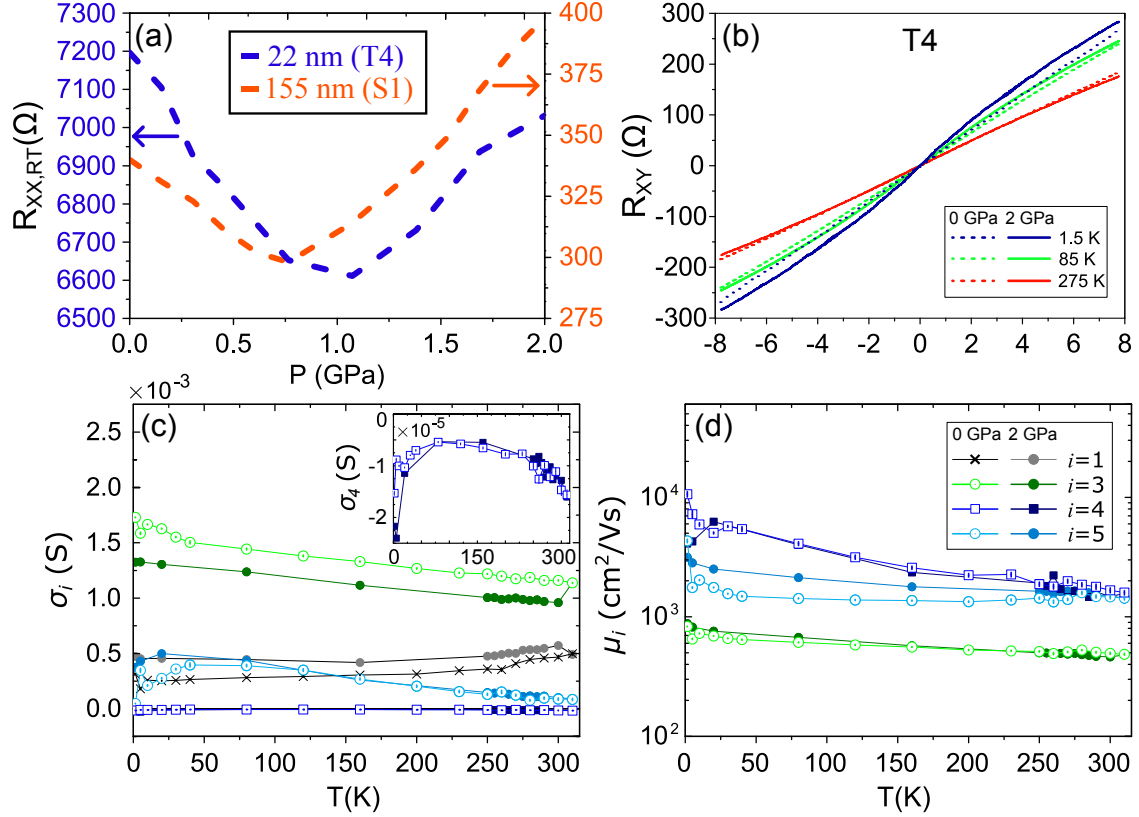

Figure S6. (a) Device resistance at room temperature during pressure application. Similar to the thick devices (orange dashed line), device T4 (blue dashed line) has a distinct minimum resistance. (b) Comparative Hall resistance curves at select temperatures for device T4 at 0 and 2 GPa. At high pressure the curves become more nonlinear, particularly at lower temperatures. (c), (d) MCT results for device T4 for  $\sigma_i$  and  $\mu_i$  contributions of the different carriers, at 0 and 2 GPa. The inset in (c) is a zoom on the electron contribution  $\sigma_4$ , and the legend in (d) applies to both panels.

flat to reliably fit using an arbitrary band edge and shifting chemical potential, presumably due to the latter being situated too far down into the valence band.

## VI. COMPRESSION IN DIFFERENT DIRECTIONS

Band structure calculations were performed to analyze the strain-dependent behavior of  $\text{ZrTe}_5$  bands close to the band gap. As mentioned in the main text, the particular manner in which the lattice constants are compressed under hydrostatic pressure has not been established with certainty. We have investigated two different pressure paths, as shown

in Fig. 1 (a) by the purple arrows, with path (1) being isotropic compression of all lattice constants, and path (2) being a vdW-only compression of the multilayer ZrTe<sub>5</sub> crystal. An enlarged part of the same strain map (see Fig. S7 (a)) shows the same two paths. In the main text we have focused on the isotropic case and compared it with the experimental results. Here we show the evolution of the gap along path (2) in comparison, concluding that the particular choice of compression path makes little difference in the end result. Along both paths, the gap  $\Delta_r$  closes and reopens with pressure, as shown in Fig. S7 (b). The vdW-only compression path requires a larger compression value to reach the gapless state. In Fig. S7 (c), however, we have scaled the compression axis along both paths to the minimum of the  $R_{xx}$  pressure dependence (at room temperature), associating it with the phase transition pressure. Here we can see that the overall evolution of the gap along path (1) and path (2) is very similar relative to the shape of  $R_{xx,RT}$  and the two paths do not significantly differ from each other.

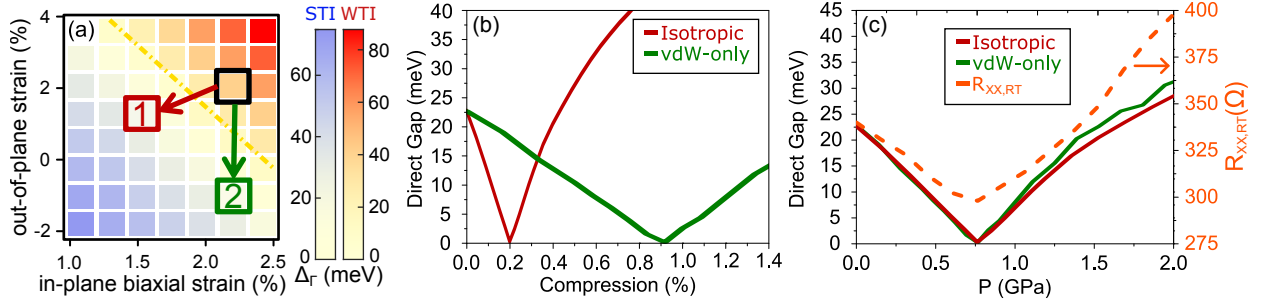

Figure S7. (a) Part of the strain map from Fig. 1 (a) of the main text, with the two different pressure paths highlighted. (b) Evolution of  $\Delta_r$  along the two different paths, on a compressive strain axis. The compression is either isotropic or vdW-only, with the latter requiring larger compression value to reach the phase transition (gapless) state. (c) Comparison of the isotropic and vdW-only paths with their minima scaled to the minimum of the  $R_{xx}(p)$  dependence of the devices, indicative of the phase transition point. There is little difference between the two compression paths in this case.

## VII. BAND STRUCTURE CALCULATION METHOD

Here we specify the details of the *ab initio* band structure calculation methodology. The optimized geometry and electronic properties of the crystal were obtained by the SIESTA implementation of DFT [4–7]. SIESTA employs norm-conserving pseudopotentials to account for the core electrons and linear combination of atomic orbitals to construct the valence states. The generalised gradient approximation of the exchange and the correlation functional was used with Perdew–Burke–Ernzerhof parametrisation [8] and the pseudopotentials optimized by Rivero *et al.* [9] with a double- $\zeta$  polarised basis set and a realspace grid defined with an equivalent energy cutoff of 350 Ry for the relaxation phase and 900 Ry for the single-point calculations. The calculated relaxed lattice parameters are very close to the experimental lattice constants obtained from powder diffraction [10, 11], differing by about 1%. The Brillouin zone integration was sampled by a  $30 \times 30 \times 18$  Monkhorst–Pack  $k$ -grid for both the relaxation and the single-point calculations. [12] The geometry optimizations were

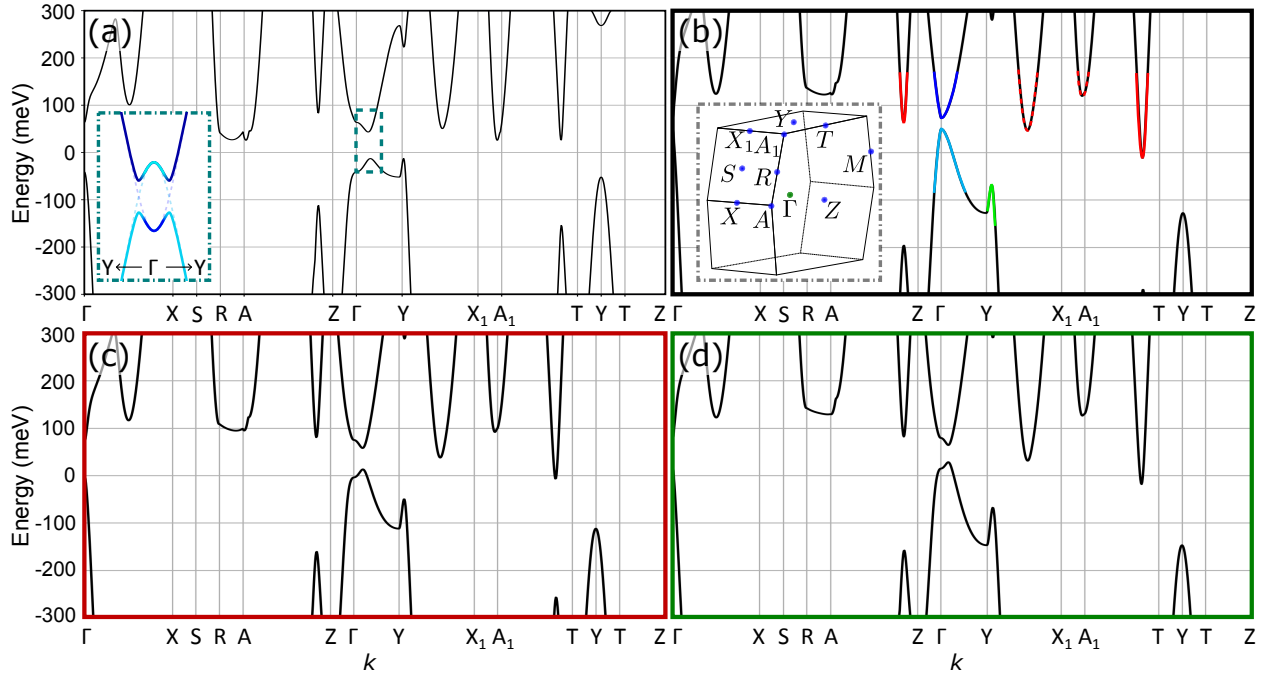

Figure S8. (a) Calculated ZrTe<sub>5</sub> band structure in the relaxed lattice constant case. Inset shows a model of the inverted bands along  $\Gamma$ -Y. (b) Band structure corresponding to the black square in Fig. 1 (a). Inset shows the high-symmetry points along the Brillouin zone. (c), (d) Band structures of the red and green squares in Fig. 1 (a), respectively.

performed until the forces were smaller than  $0.1 \text{ eV nm}^{-1}$ . The choice of pseudopotentials optimized by Rivero *et al* ensures that both the obtained geometrical structures and the electronic band properties are reliable. After the successful self consistent cycles the necessary information was obtained by the sisl tool [13]. The spin orbit coupling was taken into account in the single point calculations.

Band structures obtained for specific points on the strain map of Fig. 1 (a) are shown in Fig. S8. The relaxed lattice constants are  $a = 2.002 \text{ \AA}$ ,  $b = 7.204 \text{ \AA}$  and  $c = 13.876 \text{ \AA}$ . For comparison, the lattice constants verified by X-ray diffraction differ by no more than 1.1%, with  $a = 1.994 \text{ \AA}$ ,  $b = 7.265 \text{ \AA}$  and  $c = 13.724 \text{ \AA}$ , matching the results of Ref. [10]. Fig. S8 (a) shows the zero strain band structure, using the relaxed lattice constants. The system is in an STI phase with significant band inversion, including avoided crossing visible along the  $\Gamma$ -Y line. The inset is a model of the inverted conduction and valence bands along this line. The structure corresponding to the black square from Fig. 1 (a) is shown in Fig. S8 (b), in this case being in the WTI phase. On this panel, the band edges are highlighted with the respective colors used for the carriers in the MCT model, see Fig 4. (a). The inset is a depiction of the Brillouin Zone. Finally, Fig. S8 (c) and (d) show the band structures in the red and green squares from Fig. 1 (a), where compression has taken place in an isotropic or vdW-only fashion, respectively, starting from the black square. Both are past the topological phase transition, in an STI phase.

- 
- [1] J. Lu, G. Zheng, X. Zhu, W. Ning, H. Zhang, J. Yang, H. Du, K. Yang, H. Lu, Y. Zhang, and M. Tian, Thickness-tuned transition of band topology in  $\text{ZrTe}_5$  nanosheets, *Phys. Rev. B* **95**, 125135 (2017).
  - [2] J. Niu, J. Wang, Z. He, C. Zhang, X. Li, T. Cai, X. Ma, S. Jia, D. Yu, and X. Wu, Electrical transport in nanothick  $\text{ZrTe}_5$  sheets: From three to two dimensions, *Phys. Rev. B* **95**, 035420 (2017).
  - [3] F. Tang, P. Wang, P. Wang, Y. Gan, L. Wang, W. Zhang, and L. Zhang, Multi-carrier transport in  $\text{ZrTe}_5$  film, *Chinese Physics B* **27**, 087307 (2018).
  - [4] E. Artacho, E. Anglada, O. Diéguez, J. D. Gale, A. García, J. Junquera, R. M. Martin, P. Ordejón, J. M. Pruneda, D. Sánchez-Portal, and J. M. Soler, The SIESTA method; developments

- and applicability, *Journal of Physics: Condensed Matter* **20**, 064208 (2008).
- [5] J. M. Soler, E. Artacho, J. D. Gale, A. García, J. Junquera, P. Ordejón, and D. Sánchez-Portal, The SIESTA method for ab initio order-N materials simulation, *Journal of Physics: Condensed Matter* **14**, 2745 (2002).
  - [6] A. García, N. Papior, A. Akhtar, E. Artacho, V. Blum, E. Bosoni, P. Brandimarte, M. Brandbyge, J. I. Cerdá, F. Corsetti, *et al.*, Siesta: Recent developments and applications, *J. Chem. Phys.* **152**, 204108 (2020).
  - [7] L. Fernández-Seivane, M. A. Oliveira, S. Sanvito, and J. Ferrer, On-site approximation for spin-orbit coupling in linear combination of atomic orbitals density functional methods, *Journal of Physics: Condensed Matter* **18**, 7999 (2006).
  - [8] J. P. Perdew, K. Burke, and M. Ernzerhof, Generalized gradient approximation made simple, *Phys. Rev. Lett.* **77**, 3865 (1996).
  - [9] P. Rivero, V. M. García-Suárez, D. Pereñíguez, K. Utt, Y. Yang, L. Bellaiche, K. Park, J. Ferrer, and S. Barraza-Lopez, Systematic pseudopotentials from reference eigenvalue sets for DFT calculations, *Computational Materials Science* **98**, 372 (2015).
  - [10] H. Fjellvåg and A. Kjekshus, Structural properties of  $\text{ZrTe}_5$  and  $\text{HfTe}_5$  as seen by powder diffraction, *Solid State Communications* **60**, 91 (1986).
  - [11] Z. Tajkov, D. Nagy, K. Kandrai, J. Koltai, L. Oroszlány, P. Süle, Z. E. Horváth, P. Vancsó, L. Tapasztó, and P. Nemes-Incze, Revealing the topological phase diagram of  $\text{ZrTe}_5$  using the complex strain fields of microbubbles, *npj Computational Materials* **8**, 177 (2022).
  - [12] H. J. Monkhorst and J. D. Pack, Special points for Brillouin-zone integrations, *Phys. Rev. B* **13**, 5188 (1976).
  - [13] N. Papior, *sisl: v0.11.0* (2021).
